# Supplementary material for: Photocatalytic water splitting ability of Fe/MgO-rGO nanocomposites towards hydrogen evolution
Source: arXiv:2111.01831 source file (2022-01-03)
Supplement: Supplementary file 1 [file appendix1.tex]

\section{Supplementary Material} \label{sec:appendix}
    Here the ESI will be included.
